# Supplementary material for: MoE Jetpack: From Dense Checkpoints to Adaptive Mixture of Experts for Vision Tasks
Source: arXiv:2406.04801 source file (2024-06-07)
Supplement: Supplementary file 1 [file Appendix_hyper_parameters.tex]

\begin{table}[tbh]
    \centering
    \vspace{-3mm}
    \caption{Training settings for different datasets.}
    \vspace{2mm}
    \addtolength{\tabcolsep}{-1mm}
    \begin{tabular}{lcccc}
        \toprule
        Setting   & \makecell{Batch \\ Size} & \makecell{Warmup \\ Epochs} & \makecell{Training \\ Epochs} & \makecell{Drop \\ Path Rate} \\ 
        \midrule
        C-10    & $1024$ & $50$ & $300$ & $0.1$ \\ 
        C-100   & $1024$ & $50$ & $300$ & $0.1$ \\ 
        Pets    & $128$  & $100$ & $600$ & $0.1$ \\ 
        Flowers & $128$  & $100$ & $600$ & $0.1$ \\ 
        STL-10  & $128$  & $50$ & $300$ & $0$ \\ 
        Food101 & $1024$ & $50$ & $300$ & $0.1$ \\ 
        DTD     & $128$  & $50$ & $600$ & $0.2$ \\ 
        IN1k    & $4096$ & $50$ & $300$ & $0$ \\ 
        \bottomrule
    \end{tabular}
    \label{tab:training_settings}
\end{table}
